# Supplementary material for: Saliency Driven Image Manipulation
Source: arXiv:1612.02184 source file (2018-01-17)
Supplement: Supplementary file 1 [file supp.tex]

\pagebreak
\begin{center}
\textbf{\large Supplemental Materials}
\end{center}

\input{fig_gray.tex}
\input{fig_reducing_bg.tex}

\input{fig_different_effects.tex}
